# Supplementary material for: Finite-Time Consensus Learning for Decentralized Optimization with Nonlinear Gossiping
Source: arXiv:2111.02949 source file (2021-11-13)
Supplement: Supplementary file 1 [file appendix.tex]

\clearpage

\bibliography{ngo}
\bibliographystyle{plain}
\end{document}
